# Supplementary material for: Calliope: Automatic Visual Data Story Generation from a Spreadsheet
Source: arXiv:2010.09975 source file (2020-10-20)
Supplement: Supplementary file 1 [file supplement.tex]

\section{Fact Significance}

Fact significance is calculated based on the former auto-insights techniques \cite{tang2017extracting, ding2019quickinsights, wang2019datashot}. 
As the definition in the references, the significance measure reveals the uncommonness of an observed insight in the result set \cite{tang2017extracting}.
A meaningful fact should exhibit significant differences against a baseline which reflects common situations formed up by majority of non-insights \cite{ding2019quickinsights}.
In the following section, we state the calculation methods for each fact type using the same statements in the these references. 

% To keep the consistent with the references  \cite{tang2017extracting, ding2019quickinsights, wang2019datashot}, we let $X={x_1, x_2, ... , x_n}$ be the set of numeric values that represents the aggregated $measure$ grouped by $breakdown$ in the fact.

\paragraph{\bf Value} DataShot states ``Some data facts (e.g., Value, Aggregation) only derive values from the data simply assign it to zero. We simply assign them to zero."\cite{wang2019datashot}. In our implementation, we use the probability of the fact to calculate the significant score.

\paragraph{\bf Difference}
A significant difference between two $focus$ corresponds to a high score for Difference. 
The significance is equal to 1 when the difference is maximum.

\paragraph{\bf Proportion}
We follow the definition of \underline{Proportion} in DataShot\cite{wang2019datashot} and \underline{Attribution} in QuickInsights\cite{ding2019quickinsights}.
DataShot states ``A high proportion corresponds to a high score for Proportion".
QuickInsights states ``Attribution shows the fact that the leading value dominates (accounting for >= 50\% of) the group".
Thus we directly use the proportion as the significance of proportion. 
In addition, if the proportion is larger than 50\%, we set the significance as 1 because the focus part dominates the group.

\paragraph{\bf Trend}
We follow the definition of \underline{Trend} in DataShot and \underline{Shape Insight} in Top-K Insights\cite{tang2017extracting}.
DataShot states ``A sharp increase corresponds to a high score for Trend".
Top-K Insights states ``In business intelligence applications, data analysts are attracted to a clear rising/falling trend, whose slope is very different from 0".
The following is the method mentioned in the Top-K Insights:

We set the null hypothesis as $X$ forms a shape with a slope near 0.
Thus, the p-value should measure how surprisingly the slope differs from 0.

1. First, we fit $X$ to a line by linear regression analysis, and then compute its slope $slope$ and the goodness-of-fit value $r^{2}$.

2. we use logistic distribution to model the distributions of slopes.

3. The p-value is the probability of the slope values equal to or larger than the observed slope of the rising trend.

4. Finally, we define the significance as $S(f)=r^2\cdot (1-p)$, where the goodness-of-fit value $r^2$ is used as a weight.

\paragraph{\bf Categorization}
We follow the definition of \underline{Evenness} in QuickInsights\cite{ding2019quickinsights}.
QuickInsights states that Evenness shows that the cases where all value of a measure for a given category should be close to each other. The following is the method:

1. Perform the CHI square test for the hypothesis: the counts in each category are equal.

2. We obtain the significance as $S(f)=1-p$.

\paragraph{\bf Distribution}
The significance of distribution should reveal how surprisingly $X$ differs from the Gaussian distribution, which is the common distribution in the natuaral world.
The following is the method:

We set the null hypothesis $X$ as a power-law distribution with Gaussian noises.

1. Perform the Shapiro-Wilk test for $X$.

2. We obtain the significance as $S(f)=1-p$.

\paragraph{\bf Rank}
% Using linear regression to fit power law distribution. fit_intercept=False means y=ax, no b.
We follow the definition of \underline{Point Insight} in Top-K Insights\cite{tang2017extracting}.
Top-K Insights states ``In the business domain, the sale of products often follows a power-law distribution".
The following is the method mentioned in Top-K Insights:

We set the null hypothesis $X$ as a power-law distribution with Gaussian noises.

1. First, we sort $X$ in the descending order and obtain the maximum value $x_{max}$.

2. Then, we fit the values in $X$ to a power-law distribution if it is good fit, where the prediction errors (i.e., subtracting observed value $\hat{x_i}$ from estimated value $x_i$ , also called residuals) approximately follow Gaussian distribution.

3. Next, we determine how surprising it is that $X$ observed against the hypothesis and calculate the p-value $p$.

4. Finally, we obtain the significance as $S(f)=1-p$.

\paragraph{\bf Association}
We follow the definition of \underline{Correlation} in QuickInsights\cite{ding2019quickinsights}.
The following is the method mentioned in the QuickInsights:

The significance of two $measure$ is defined based on testing using Student's t-distribution with Pearson's correlation coefficient $r$.

1. Specify the null and alternative hypotheses.

2. Calculate the value of test statistic: $t=r \sqrt{\frac{n-2}{1-r^{2}}}$.

3. Use the resulting test statistic $t$ to calculate the p-value, which is determined by referring to a t-distribution with n-2 degrees of freedom.

4. The p-value is translated into significance. The lower the p-value, the higher the significance.

\paragraph{\bf Extreme}
We follow the definition of \underline{Outstanding No.1} and \underline{Outstanding Last} in QuickInsights\cite{ding2019quickinsights}.
The following is the method mentioned in the QuickInsights:

Take Outstanding No. 1 as an example.
Given a group of non-negative numerical values {x} and their biggest value $x_{max}$ , the significance of $x_{max}$ being Outstanding No.1 of $X$ is defined based on the p-value against the null hypothesis of $X$ obeys an ordinary long-tail distribution.

1. We sort $X$ in descending order;

2. We assume the long-tail shape obeys a power-law function. Then we conduct regression analysis for the values in $X$. $x_{max}$ using power-law functions, where i is an order index and in our current implementation we fix $\beta = 0.7$ in the power-law fitting;

3. We assume the regression residuals obey a Gaussian distribution. Then we use the residuals in the preceding regression analysis to train a Gaussian model $H$;

4. We use the regression model to predict $x_{max}$ and get the corresponding residual $R$;

5. The p-value will be calculated via $P(R|H)$.

\paragraph{\bf Outlier} We follow the definition of \underline{Outlier} in DataShot and QuickInsights\cite{wang2019datashot, ding2019quickinsights}.
Because of no exact method mentioned in these papers, we use the a statistic method Grubbs' test, which is a commonly used way to detect outliers.

%1. Normalized $X$ into z-score.
1. The first step is to quantify how far the outlier is from the others. We calculate The Grubbs test statistic $G$ as the largest absolute deviation from the sample mean in units of the sample standard deviation.
%For each instance $x$, its z-score is defined as $Z = \frac{\left|x - \bar x\right|}{SD}$.

2. The hypothesis of no outliers at a certain significance level is rejected if the calculated $G$ is greater than the corresponding critical value in the table, which have been tabulated for the Grubbs test statistic. 
%We assume the z-score obey a Gaussian distribution. Then we use the z-score to train a Gaussian model $H$;

3. If there exist at least an outlier and the p-value is small, we can conclude that the deviation of the outlier from other values is statistically significant. The lower the p-value is, the higher the significance is. Hence We obtain the significance as $S(f)=1-p$. 

4. Otherwise, If the hypothesis of no outliers is accepted which means there is no outlier in the sample, the significance is equal to 0.
% Grubbs' test only tests the most extreme value in the sample. Thus, we calculate $Z$ for all values, but only calculate a p-value for Grubbs' test from the largest value of $Z$. 
% The p-value will be calculated via $P(outlier|H)$.

\section{An Example of the Algorithm}

To explain the algorithm, we provide a concrete example in which the process of creating a 3-facts story is explained in detail. Here we use a simplified spreadsheet about the deaths of COVID-19 in China from March 1st to March 21st as a running example. The spreadsheet contains 3 columns including Date(temporal), Province(categorical), and Deaths(numerical). 

Initially, the algorithm generates a set of random facts according to the preliminary survey as the first fact, such as the Value fact “The value of the \underline{total deaths} is 423” (\textbf{F1}), the Trend fact “The trend of the \underline{total deaths} over \underline{dates} is decreasing” (\textbf{F2}), and the Categorization fact “The data contains 32 \underline{provinces}”(\textbf{F3}). According to the importance score, the \textbf{F2} is chosen as the root of the tree.

\begin{figure}[htb]
    \centering
    \includegraphics[width=\linewidth]{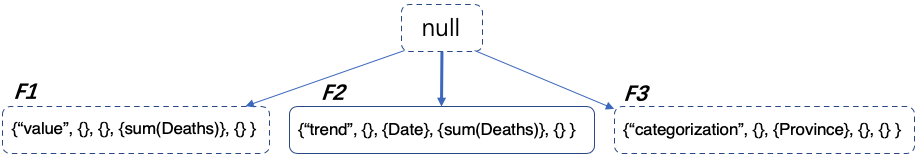}
    % \caption{fig1}
\end{figure}

In the next, the algorithm begins an iterative process with 4 major steps: selection, expansion, simulation, and back-propagation. 

\begin{itemize}
    \item {\bf Selection}: At first, it finds a fact with the largest reward in the tree. In the current stage, \textbf{F2} is picked because it is the only fact in the tree. 

    \item {\bf Expansion}: Secondly, the algorithm expands a set of data facts from the Trend fact according to the different logical relation. For example, a contrast relation may lead to the Trend fact “The \underline{total deaths} over \underline{dates} shows an increasing trend when \underline{the province is Hong Kong}” (\textbf{F4}), an elaboration relation can lead to the Extreme fact “The maximum value of the \underline{total deaths} is 42 when \underline{the date is 2020/3/2}” (\textbf{F5}), and a similarity relation can trigger the Distribution fact “The distribution of the \underline{total deaths} over different \underline{provinces} shows an overview” (\textbf{F6}).

    \item {\bf Simulation}: Thirdly, the algorithm starts to simulate from all the expanded facts (\textbf{F4}, \textbf{F5} and \textbf{F6}). In each simulation process, the algorithm tries to explore the design space and find a path with the largest reward. 

    \item {\bf Back-propagation}: The rewards of the facts in the tree are updated after each simulation. In this example, the algorithm finds that choosing \textbf{F5} will lead to a path with the largest reward. Thus, it updates the reward $\Delta$ in the path (\textbf{F2}, \textbf{F5}) during back-propagation.
\end{itemize}

\begin{figure}[htb]
    \centering
    \includegraphics[width=\linewidth]{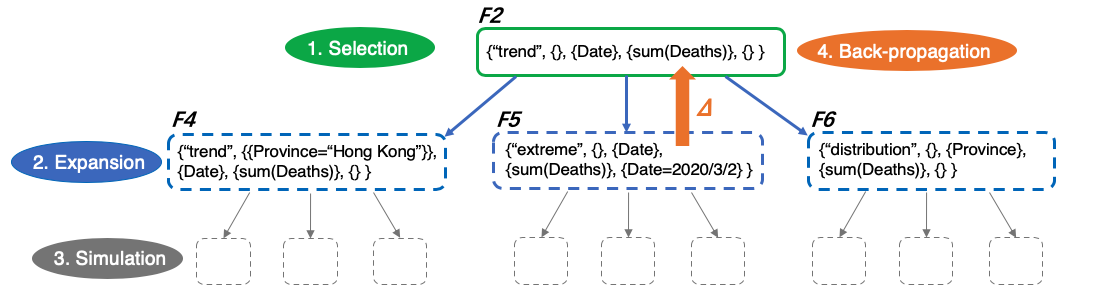}
    % \caption{fig1}
\end{figure}

% \begin{figure*}[ht]
%     \centering
%     \includegraphics[width=0.86\linewidth]{figures/example-step-2.png}
%     \vspace{-0.5em}
%     \caption{Two data story examples.} 
%     \label{fig:casestudy}
% \end{figure*}

Now \textbf{F5} is the node with the largest reward in the tree. Thus, it will be selected as the beginning node in the next iteration. A new Distribution fact \textbf{F7} is expanded during the similar search process. The algorithm stops when the goal is fulfilled. In the end, the path (\textbf{F2}, \textbf{F5}, \textbf{F7}) with the highest reward is the best story in the tree.

\begin{figure}[htb]
    \centering
    \includegraphics[width=\linewidth]{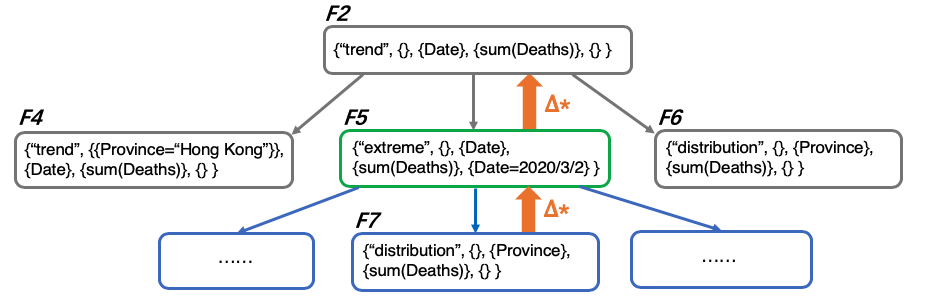}
    % \caption{fig1}
\end{figure}

% \begin{figure*}[t]
%     \centering
%     \includegraphics[width=0.8\linewidth]{figures/example-step-3.png}
%     \vspace{-0.5em}
%     \caption{Two data story examples.} 
%     \label{fig:casestudy}
% \end{figure*}

The following figure is the storyline of the final 3-facts data stories. It illustrates that the trend of daily mortality in China was decreasing in March (Fact 1). In particular, the largest number was 42 occurred on March 2nd (Fact 2). Finally, the distribution shows that Hubei was the most dangerous province (Fact 3).

\begin{figure}[htb]
    \centering
    \includegraphics[width=0.82\linewidth]{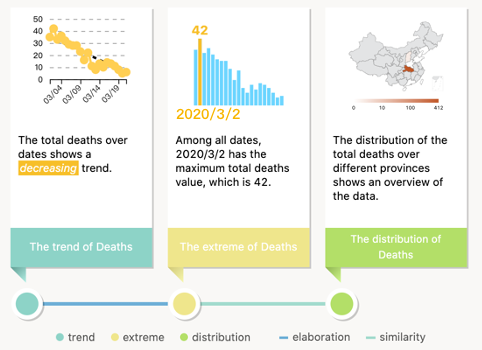}
    % \caption{result} 
\end{figure}
